# Supplementary material for: Category-Specific Object Reconstruction from a Single Image
Source: arXiv:1411.6069 source file (2015-05-06)
Supplement: Supplementary file 1 [file PointCloudModelsSupplementary.tex]

%\textcolor{red}{ 'occluding contours' to 'silhouettes', shape model as 'set' of points to matrix, more intuition for optimization }

\subsection{Shape Model}
We learn a shape model $M = (\overline{S},V)$ comprising a mean shape $\overline{S}$ and deformation bases $V = \{ V_1,.,V_K \} $. An explicit point coordinate based representation is used and therefore $\overline{S}, V_i \in \mathbb{R}^{N \times 3}$. Our basis shape model represents a shape $S$ as a the mean shape deformed by a linear combination of the deformation bases i.e. $S = \overline{S} + \underset{k}{\sum}\alpha_{k} V_k$. The expressive power of our model is the similar to PCA as they both cover a $K$ dimensional subspace of $\mathbb{R}^{N \times 3}$ using $K$ basis vectors (though we do not enforce orthogonality of deformation basis as the various sematically meaningful deformation modes across a category are not necessarily orthogonal).

\subsection{Inputs}
We learn the shape model using training set $T:\{(O^i,P^i)\}$ where $O^i$ is the corresponding silhouette and $P^i$ is the function to project points from the world coordinates to image coordinates. The silhouette for an instance is represented as the coordinates of the set of boundary points in the image frame. To infer the shape $S$ for new instance, we require the same input - $(O,P)$ (it's silhouette and projection function). Note that the $P^i$ we obtain using NRSfM corresponds to orthographic projection but our algorithm to infer shape models can handle perspective projections as well.

\subsection{Energy Formulation}
We formulate an objective function based on three properties which a proposed solution should intuitively satisfy  - 1)\textit{Silhouette Consistency:} the shape inferred for an instance does not project outside its silhouette. 2) \textit{Silhouette Coverage:} every point on the silhouette is adjacent to at least some (say $m$)  points on the projected model-induced shape for the instance. 3) \textit{Local Consistency:} distance to a point's nearest neighbors is small and neighboring points have similar deformations. We capture these properties by defining corresponding energy terms as follows (here $\Delta(Q,p,k)$ corresponds to the average distance of $p$ to its nearest $k$ neighbors in $Q$):

\begin{gather}
 \label{eq:local_con}\text{Local Consistency: }E_{L}(\bar{S},V)=\underset{i}{\sum}\underset{j\epsilon N(i)}{\sum}(\|\bar{S}_{i}-\bar{S}_{j}\|^2 +\underset{k}{\sum}\|V_{ki}-V_{kj}\|^2) \\
 \label{eq:sil_con} \text{Silhouette Consistency: }E_{S}(S,O,P)=\underset{p \in P(S)\setminus Mask(O)}{\sum}\Delta(O,p,1)^{2}\\
  \label{eq:sil_cov}\text{Silhouette Coverage: }E_{C}(S,O,P)=\underset{p\epsilon O}{\sum}\Delta(P(S),p,m)^2
\end{gather}

Equation~\eqref{eq:sil_con} penalizes the projected points according to the Chamfer distance field of the mask corresponding to silhouette $O$. Equation~\eqref{eq:sil_cov} penalizes large discrepancies from every boundary pixel to its $m$ nearest neighbors in the projected shape.  We use the objective in equation \ref{eq:formulation} to learn a shape model $M = (\overline{S},V)$ such that the shapes inferred using the model for all instances in the training set satisfy the above properties while penalizing the amount of deformation to regularize the objective.

\begin{equation}
\label{eq:formulation}
\underset{\bar{S},V,\alpha}{\min} E_{L}(\bar{S},V)+\underset{i}{\sum}(\lambda_{1}E_{S}(S^{i},O^{i},P^{i})+\lambda_{2}E_{C}(S^{i},O^{i},P^{i})+\lambda_3\underset{k}{\sum}(\|\alpha_{ik}V_k\|_F^{2}))
\end{equation}

where 

\[
S^i = \overline{S} + \underset{k}{\sum}\alpha_{ik} V_k \text{  : Shape for }  i^{th} \text{ training instance}
\]

\subsection{Learning and Inference}
As can be seen in fig.~\ref{fig:basisShapesModel}, the shape models learned using our formulation are able to model the coarse level category shapes as well as the intra-class variation using the mean shapes and deformation bases respectively.

\begin{figure}[htb!]
\centering
\begin{subfigure}{.45\textwidth}
  \includegraphics[width=\linewidth, trim=8 8 8 8,clip]{figures/meanShapes.pdf}
  \caption{Mean shapes for chair, aeroplane, bicycle and car classes.}
  \label{fig:meanDense}
\end{subfigure}%
\hfill
\begin{subfigure}{.45\textwidth}
  \includegraphics[width=\linewidth]{figures/aeroplaneDeformations.jpg}
  \caption{Deformation modes for aeroplanes.}
  \label{fig:denseDeformations}
\end{subfigure}
\caption{Our basis shapes model learns a mean shape and a deformation basis for each class. a) Learned mean shapes for various categories. b) Mean shape for aeroplane deformed according to the learned deformations bases. }
\label{fig:basisShapesModel}
\end{figure}
To infer the shape for a novel image using the learned model $M=(\bar{S},V)$, we solve for the deformation weights $\alpha$ by optimizing equation~\eqref{eq:formulation} wrt $\alpha$ for fixed $\bar{S},V$.

\subsection{Initialization}
Our training objective is non-convex and  non-smooth and is susceptible to local minima. We follow the suggestion of \cite{esteban2004snake} and initialize our mean shape with the visual hull computed using \textit{all} training instances. The deformation bases and deformation weights are initialized randomly.

\subsection{Optimization Implementation}
To address the scale ambiguity between $V$ and $\alpha$ in our formulation, we restrict $\|V_k\|_F$ to be a constant. The mean shape and deformation basis are inferred via block-coordinate descent on the objective using sub-gradient computations over the training set.
