# Supplementary material for: Category-Specific Object Reconstruction from a Single Image
Source: arXiv:1411.6069 source file (2015-05-06)
Supplement: Supplementary file 2 [file VisualHullModelsSupplementary.tex]

Parametric models with simple deformations might not sufficiently capture large intra-class variance which is frequently present in some categories. Allowing complex deformations, on the other hand, would result in a significant increase in the computational complexity as well as the possibility of overfitting. We explore whether representing category shapes via multiple learned prototypes can alleviate these issues. We propose to learn a representative set of 3D prototypes for a category employing variations of visual hull techniques that we make more robust to intra-class variation and noisy camera estimates.

A key observation which enables this approach is that an estimate of a coarse rotation invariant shape parameter allows grouping of visually similar instances into ``visual clusters". Deriving our prototypes from these visual clusters provides an effective way of modeling the various modes of the distribution underlying the shapes of an object category. Formally, we infer our shape model from a training set $T:\{(O^i,P^i,\alpha^i)\}$, where the quantities $O_i$ and $P_i$ are as described in the previous section. The additional input $\alpha^i$ corresponds to the coarse rotation invariant shape parameter which in our implementation is the deformation weight vector obtained using the NRSfM algorithm. Note that the proposed approach can exploit any coarse shape parameter (e.g. simple cues based on the silhouette shape).

\subsubsection{Learning:}
\begin{figure}[htb!]
\centering
\begin{minipage}{.45\textwidth}

  \includegraphics[width=.45\linewidth]{figures/visClusters1.jpg}
  \label{fig:VisCluster1}
\quad
%\begin{subfigure}{.22\textwidth}
  \includegraphics[width=.45\linewidth]{figures/visClustersShape1.jpg}
  \label{fig:VisShape1}
%\end{subfigure}

%\begin{subfigure}{.22\textwidth}
  \includegraphics[width=.45\linewidth]{figures/visClusters2.jpg}
  \label{fig:VisCluster2}
%\end{subfigure}%
\quad
%\begin{subfigure}{.22\textwidth}
  \includegraphics[width=.45\linewidth]{figures/visClustersShape2.jpg}
  \label{fig:VisShape2}
%\end{subfigure}
\vspace{7pt}
  
\caption{Learned prototype shapes corresponding to different visual clusters.}
\label{fig:visClusterShapes}
\end{minipage}
\hspace{0.05\textwidth}
%\vspace*{\fill}
%\begin{center}
\begin{minipage}{.45\textwidth}

\centering
 \includegraphics[width = \linewidth]{figures/visHullPlanes.jpg}
%\vspace{-5}
\caption{Illustration of visual cones induced by silhouettes.}
\label{fig:visHullPlanes}

\end{minipage}
%\end{center}

%\vfill
\end{figure}

%\begin{figure}[htb!]
%\centering
% \includegraphics[scale = 0.2]{figures/visHullPlanes.jpg}
%\caption{Illustration of visual cones induced by silhouettes.}
%\label{fig:visHullPlanes}
%\end{figure}

We represent the shape model $M = \{ (\bar{S_k},\alpha_k) | k=1..K\}$ as a set of volumetric shape representations $\bar{S_k}$ and associated shape parameters $\alpha_k$. The individual prototype $\bar{S_k}$ is learned from the corresponding visual cluster and the associated shape parameter $\alpha_k$ represents the mean deformation parameter for the corresponding cluster.

In fig.~\ref{fig:visClusterShapes}, we visualize some training instances and their ``visual cones" - a visual cone is the volume that projects inside the silhouette under the corresponding orthographic transformation. The visual hull approach for learning a shape model is to take the intersection of all the visual cones and the object volume is then represented as a binary value associated with each voxel. We use an extensible representation based on the truncated signed distance function (TSDF) which is a field over voxel space such that a level set describes the object surface. A TSDF represents the signed distances of points from a surface and the distances are truncated at some minimum and maximum thresholds. We denote a TSDF $S$ whose values are restricted between $[l,L]$ as $S[l,L]$. Thus the prototype $\bar{S_k}$ visual hull from the associated visual cluster $C_k$ is simply
\begin{equation}
\label{eq:VisLearning}
\bar{S_k} = \underset{i \in C_k}{\sum}S^i[0,\infty]
\end{equation}
where $S_i[0,\infty]$ is the TSDF representing the distances from the surface of the visual cone for  $O^i$ under transformation $P^i$. We prefer the TSDF representation because it can be easily extended to handle variations and noise as we describe later. Fig.~\ref{fig:visHullPlanes} shows some visual clusters and the corresponding prototype models that we learn.

\subsubsection{Inference:}
Given an instance $I = (O,P,\alpha)$, we hypothesize that its dense shape would be similar to the shape of the instances in the most similar visual cluster in our model $M = \{ (\bar{S_k},\alpha_k)\}$. Thus, we find its closest cluster $C_j$ in the training set and combine the shape information obtained using the silhouette for the particular instance with the prototype model of $C_j$. We first compute the TSDF $S[0,\infty]$ for the particular instance using $(O,P)$. This volumetric representation is then updated according to equation \ref{eq:inferenceVis} to infer the dense shape for the given instance.
\begin{equation}
\label{eq:inferenceVis}
S \leftarrow S + \lambda \bar{S_j}
\end{equation}
\subsubsection{Allowing for Intra-class Variations and Camera Estimation Error:}
The approach described above learns the visual hull for each visual cluster. However, this may not be the desirable as our camera estimates are not perfect and a visual cluster does not exactly correspond to an instance. We suggest two modifications to make our method more robust -
\begin{itemize}
\item Instead of using a minimum truncation value 0 for the TSDF computations, we allow a small negative value. This results in learned/inferred shapes which differ from the visual hull approach by allowing us to retain the voxels which are consistent with a majority of the instances and violate very few constraints, presumably due to shape variations or noisy camera estimates.
\item The distribution of views for an object class is often non-uniform and to account for this, we modify the learning in equation \ref{eq:VisLearning} to assign an importance weight to each instance. Since we aim to negate the viewpoint bias using these weights, we first cluster the camera viewpoints within each visual cluster. The weight for each instance is then assigned to be inversely proportional to the size of its corresponding viewpoint cluster to normalize for the view distribution.
\end{itemize}
